# Supplementary material for: C3G: Learning Compact 3D Representations with 2K Gaussians
Source: arXiv:2512.04021 source file (2026-04-28)
Supplement: Supplementary file 4 [file n_view_feature_lifting.tex]

\begin{table*}[t]
\centering
\caption{\textbf{multi-view extension of feature lifting.} }
\label{suptabmulti-view feature}
\resizebox{0.75\linewidth}{!}{
\begin{tabular}{l|ccc|ccccc}
\toprule
\multirow{2}{*}{Methods} & \multirow{2}{*}{\shortstack{\shortstack{feed\\forward}}} & \multirow{2}{*}{\shortstack{Number of\\inputs}} & \multirow{2}{*}{\shortstack{Number of\\forward}} & \multicolumn{5}{c}{Lseg~\cite{li2022language}} \\
& & & & mIoU$\uparrow$ & Acc.$\uparrow$ & PSNR$\uparrow$ & SSIM$\uparrow$ & LPIPS$\downarrow$ \\
\midrule
Feature-3DGS~\cite{zhou2024feature} & \ding{55} & N & - & 0.379& 0.644& 19.83& 0.684& 0.357\\
CF$^3$~\cite{lee2025cf3}& \ding{55} & N & - & 0.376& 0.657& 20.04& 0.691& 0.359\\
\midrule
Ours & \ding{51} & 2 & N & 0.513& 0.783& 23.89& 0.770& 0.285\\
Ours & \ding{51} & 24 & 1 & & & & & \\
\bottomrule
\end{tabular}}
\end{table*}
