# Supplementary material for: C3G: Learning Compact 3D Representations with 2K Gaussians
Source: arXiv:2512.04021 source file (2026-04-28)
Supplement: Supplementary file 5 [file probe3d_fit3d.tex]

\begin{table}[t]
\centering
\caption{\textbf{Correspondence estimation on ScanNet.} We evaluate PCK@10px across two images captured from different angle. Our feature aggregation significantly improves correspondence accuracy with the DINOv2-Base backbones.}
\label{suptab:correspondence}
\resizebox{\linewidth}{!}{
\begin{tabular}{l|cccc|c}
\toprule
Methods & $\theta_{0}^{15}$ & $\theta_{15}^{30}$ & $\theta_{30}^{60}$ & $\theta_{60}^{180}$ & Avg. \\
\midrule
DINOv2-Base~\cite{oquab2023dinov2} & 36.9& 29.2& 19.3& 9.9& 23.8\\
FiT3D~\cite{yue2024improving} & 40.9& 32.1& 22.0& 13.9& 27.2\\
% DINOv2-base~\cite{oquab2023dinov2} + AnyUp~\cite{wimmer2025anyup}& 36.2 & 28.6 & 19.7 & 10.9 & 23.9\\
DINOv2-Base~\cite{oquab2023dinov2} + Ours & \textbf{92.9} & \textbf{88.4} & \textbf{70.5} & \textbf{22.2} &  \textbf{68.5}\\
\bottomrule
\end{tabular}}
\vspace{-10pt}
\end{table}
