# Supplementary material for: C3G: Learning Compact 3D Representations with 2K Gaussians
Source: arXiv:2512.04021 source file (2026-04-28)
Supplement: Supplementary file 6 [file upsampling.tex]

\begin{table}[t]
\centering
\caption{\textbf{Correspondence estimation on ScanNet with upsampled feature.} We evaluate PCK@10px across two images captured from different angle. Our feature aggregation significantly improves correspondence accuracy with the DINOv2-Base, DINOv2-Large and DINOv3-Large backbones.}
\label{suptab:upsampler}
\resizebox{\linewidth}{!}{
\begin{tabular}{l|cccc|c}
\toprule
Methods & $\theta_{0}^{15}$ & $\theta_{15}^{30}$ & $\theta_{30}^{60}$ & $\theta_{60}^{180}$ & Avg. \\
\midrule
DINOv2-Base~\cite{oquab2023dinov2} & 36.9& 29.2& 19.3& 9.9& 23.8\\
DINOv2-Base~\cite{oquab2023dinov2} + AnyUp~\cite{wimmer2025anyup}& 36.2 & 28.6 & 19.7 & 10.9 & 23.9\\
DINOv2-Base~\cite{oquab2023dinov2} + Ours & \textbf{92.9} & \textbf{88.4} & \textbf{70.5} & \textbf{22.2} &  \textbf{68.5}\\
\midrule
DINOv2-Large~\cite{oquab2023dinov2} & 36.6& 24.0& 19.0& 12.7& 23.1\\
DINOv2-Large~\cite{oquab2023dinov2} + AnyUp~\cite{wimmer2025anyup}& 39.4& 25.5& 19.1& 14.0& 24.5\\
DINOv2-Large~\cite{oquab2023dinov2} + Ours & \textbf{94.2}& \textbf{89.0}& \textbf{70.5}& \textbf{21.0}& \textbf{68.7}\\
\midrule
DINOv3-Large~\cite{simeoni2025dinov3} &  54.9& 44.3& 32.1& 19.3& 37.7\\
DINOv3-Large~\cite{simeoni2025dinov3} + AnyUp~\cite{wimmer2025anyup}& 48.4& 34.8& 27.1& 16.8& 31.8\\
DINOv3-Large~\cite{simeoni2025dinov3} + Ours & \textbf{94.2}& \textbf{89.1}& \textbf{70.8}& \textbf{20.9}& \textbf{68.8}\\
\bottomrule
\end{tabular}}
\vspace{-10pt}
\end{table}
